# Supplementary material for: Robust Counterfactual Explanations on Graph Neural Networks
Source: arXiv:2107.04086 source file (2022-07-12)
Supplement: Supplementary file 1 [file I_Discussion.tex]

\section{Code}
\label{sec:apx_disc}
We make our code available as part of the supplemental material to the reviewers for better replication of the results.
